# Supplementary material for: Additive manufacturing of a 3D-segmented plastic scintillator detector for tracking and calorimetry of elementary particles
Source: arXiv:2312.04672 source file (2024-06-12)
Supplement: Supplementary file 1 [file Supplementary.tex]

\section{Supplementary Information}
\label{sec:supplementary_info}

\subsection*{blablabla}
